# Supplementary material for: Feedback-tuned noise-resilient gates for encoded spin qubits
Source: arXiv:1606.01897 ancillary file (2016-06-06)
Supplement: Supplementary file 1 [file supp.pdf]

# Supplementary Information: Feedback-tuned noise-resilient gates for encoded spin qubits

Pascal Cerfontaine*,[1] Tim Botzem*,[1] Simon Sebastian Humpohl,[1]
Dieter Schuh,[2] Dominique Bougeard,[2] and Hendrik Bluhm[1]
[1]*JARA-Institute for Quantum Information, RWTH Aachen University, D-52074 Aachen, Germany*
[2]*Institut für Experimentelle und Angewandte Physik,*
*Universität Regensburg, D-93040 Regensburg, Germany*
**These authors contributed equally to this work*
(Dated: June 4, 2016)

## SUPPLEMENTARY INFORMATION

Supplementary text (Sections S.1.-S.7.)

Supplementary figures (S.1. to S.5.)

Supplementary tables (S.1. to S.5.)

References

## CONTENTS

S.1. Experimental setup 1

S.2. System characterization 1
A. Exchange pulses 1
B. Noise 2

S.3. Optimal pulses 3
A. Bloch sphere convention 3
B. Numerical pulse optimization 3
C. Fidelity estimation 3

S.4. Readout and initialization 4
A. Pulses 4
B. Data acquisition 4
C. Data postselection 5
D. Mapping state preparation to measurement errors 5

S.5. Readout calibration 5
A. Self-consistent state tomography 5
B. Benchmarking 5
C. GAMBIT 6

S.6. GAMBIT 6
A. Error syndromes 6
B. Insensitivity to measurement errors 7
C. Feedback loop 7
D. Convergence 8

S.7. Gate benchmarks 8
A. Self-consistent state tomography 8
B. Randomized benchmarking and leakage 9
C. Error amplification 10

## S.1. EXPERIMENTAL SETUP

Our sample and electrical setup are the same as in supplementary Ref. 1.

Hence, the S-$T_0$ qubit is defined in a GaAs/$Al_{0.69}Ga_{0.31}$As heterostructure with Si-$\delta$-doping 50 nm below the surface. Since a spacer layer of 40 nm is added on top, the 2DEG is located 90 nm below the surface. The gate layout (Fig. 2b) is the same as in supplementary Ref. 2 with two dedicated RF gates for high-frequency qubit operations like initialization, readout and gate operations while DC gates are used for static tuning of the qubits.

In our electrical setup, we use separate DC and RF control gates to avoid pulse distortions from bias tees, resulting in a nearly flat frequency response of the RF gates from DC to beyond 100 MHz. The qubit is defined and tuned by applying static voltages on the order of 1 V to the DC gates, while we use RF pulses from a Tektronix AWG5014C arbitrary waveform generator (AWG) on the order of 1 mV (after attenuation) for qubit manipulation. The RF gates are DC-coupled to the AWG with 43 dB attenuation.

## S.2. SYSTEM CHARACTERIZATION

### A. Exchange pulses

For system characterization we measure the AWG response through coaxial cables and attenuators. We use the AWG to apply a long, nominally rectangular pulse to the RF lines, and measure the signal that arrives just before the printed circuit board (PCB), where the sample is mounted. The measured step response includes the effect of attenuators and coaxial cables but no signal distortions due to the PCB and the sample itself. From the step response we obtain a filter describing the behavior of our system. Applying this filter to arbitrary piece-wise constant pulses reproduces the actual signal very accurately as shown in Fig. S.1.

Parameters for the experimentally motivated model $J(\epsilon) = J_0 \exp(\epsilon/\epsilon_0)$ from supplementary Ref. 3 are fitted from the oscillation frequencies of free induction decay (FID) experiments at different $\epsilon$ as in supplementary

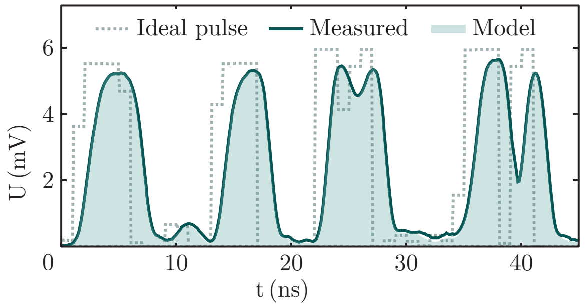


FIG. S.1. **Pulse model.** A filter based on the step response of our system is applied to nominally piece-wise constant pulses (dashed line) to predict the actual signal arriving at the PCB where the GaAs sample is mounted. Except for long-time transients (not shown) the actual signal (solid line) is accurately reproduced by the model (shaded area).

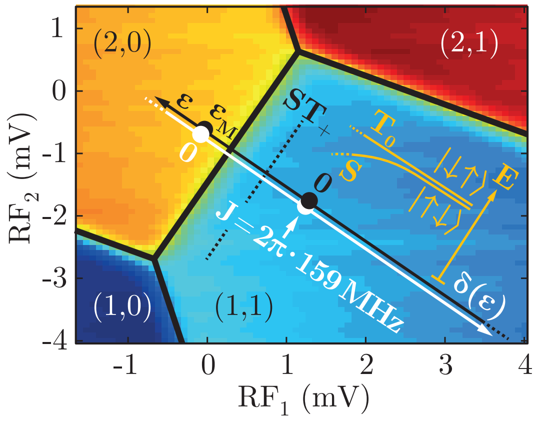


FIG. S.2. **Charge stability diagram.** Different charge occupations are indicated as a function of both RF gate voltages by $(n, m)$ with $n$ ($m$) electrons in the left (right) dot. $\delta = \epsilon_M - \epsilon$ (white) denotes the distance between the measurement point at $\epsilon_M$ and the point given by the detuning $\epsilon$ (black). $\epsilon = 0$ is defined as the point where $J(\epsilon) = 2\pi \cdot 159$ MHz. For large $\epsilon$ (low $\delta$) the exchange interaction is turned on, as indicated in the orange energy diagram. The approximate position of the S-$T_+$ transition is indicated by a dashed line.

Ref. 3, where $\epsilon$ describes the voltage change on each RF gate. We fix $J_0 = 2\pi \cdot 159$ MHz so that $\epsilon = 0$ is always defined as the point where $J(\epsilon) = 2\pi \cdot 159$ MHz. This is convenient for describing gate operations as these depend primarily on the magnitude of $J$, but the exact gate voltages where $J$ has a certain value can vary with dot tuning.

To describe this variation, we define a second frame of reference $\delta = \epsilon_M - \epsilon$. Here, $\epsilon_M$ is the position of the measurement point in the $(2,0)$ charge configuration as shown in Fig. S.2 and corresponds to $\delta = 0$. Even if the distance of the measurement point from the $(2,0)-(1,1)$ charge transition remains the same, typically around 0.25 mV, the exact value of $\epsilon_M$ depends on dot tuning since $\epsilon = 0$ is defined as the point where $J(\epsilon) = 2\pi \cdot 159$ MHz. This leads to shifts of the $\epsilon$ coordinate system when the point where $J = 2\pi \cdot 159$ MHz moves. We find that $\epsilon_M$ varies between 0.7 mV and 1.1 mV. Likewise, $\epsilon_0$ can take on values between 0.2 mV and 0.5 mV.

### B. Noise

In addition to the characterization of $J(\epsilon)$ and the step response of our setup, we extract approximate hyperfine and charge noise levels from free induction decay (FID) and spin echo (SE) experiments. For hyperfine noise, we find $T_2^* = 80$ ns and $T_2^{\text{echo}} = 13$ µs as in supplementary Ref. 1, with $\Delta B_z$ stabilized at $2\pi \cdot 61.6$ MHz by dynamic nuclear polarization[4]. These values are smaller than $T_2^* = 94$ ns and $T_2^{\text{echo}} = 30$ µs reported in supplementary Ref. 4. Instead of measuring $T_2^*$, we can also measure the fluctuations in $\Delta B_z$ directly. For a variety of dot tunings, which affect the effectiveness of the dynamic nuclear polarization pulses[4], we find standard deviations between $\sigma_{\Delta B_z} = 2\pi \cdot 2.2$ MHz and $\sigma_{\Delta B_z} = 2\pi \cdot 3.4$ MHz (after removing jumps away from the set point of $\Delta B_z$). In consideration of $T_2^{\text{echo}} \gg T_2^*$ and the slow initial decay of the Hahn echo coherence, we treat hyperfine noise as quasistatic[5] throughout this work.

For charge noise, we similarly perform FID and SE experiments at $J(\epsilon) = 2\pi \cdot 61$ MHz, yielding $T_2^* = 90$ ns and $T_2^{\text{echo}} = 183$ ns. For these FID and SE experiments we also determined $\epsilon_0 = 0.4$ mV and $\epsilon_M = 1.0$ mV so that we can approximately calculate the charge noise sensitivity in our device at $J(\epsilon) = 2\pi \cdot 61$ MHz to $dJ/d\epsilon = 2\pi \cdot 151$ MHz/mV. Based on these measurements we estimate that our sample suffers from much larger charge noise compared to supplementary Ref. 3, where $T_2^* \approx 100$ ns and $T_2^{\text{echo}} \approx 7.5$ µs were measured for $J \approx 2\pi \cdot 85$ MHz, which corresponds to a similar charge noise sensitivity $dJ/d\epsilon \approx 2\pi \cdot 150$ MHz/mV.

We use the relation

$$T_2^* = \frac{\sqrt{2}}{\sigma_\epsilon dJ/d\epsilon} \qquad \text{(S.1)}$$

given in supplementary Ref. 6 to calculate our sample's charge noise standard deviation to $\sigma_\epsilon = 1.66 \times 10^{-5}$ V. To deduce the amplitude $S_\epsilon^0$ of the high-frequency noise spectrum from $T_2^{\text{echo}}$, we assume that the noise spectrum can be described by $S_\epsilon(f) = S_\epsilon^0/f^\beta$ with $\beta = 0.7$ as measured in supplementary Ref. 3 for frequencies 50 kHz $\leq f \leq$ 1 MHz. For the purpose of calculating gate fidelities in Sec. S.3 C, we extrapolate the spectrum to follow the same power law for $f > 1$ MHz. Due to the proportionality

$$T_2^{\text{echo}} \propto \left(\frac{dJ}{d\epsilon}\right)^{-2/(\beta+1)} \qquad \text{(S.2)}$$

given in supplementary Ref. 6, we can estimate the amplitude of the high-frequency charge noise spectrum

by relating our measurements of $T_2^{\text{echo}}$ and $dJ/d\epsilon$ to those from supplementary Ref. 3, which were given as $T_2^{\text{echo}} \approx 7.5\,\mu\text{s}$, $dJ/d\epsilon \approx 2\pi \cdot 150\,\text{MHz/mV}$ and $\sqrt{S_\epsilon^0} = 2.8 \times 10^{-8}\,\text{V}/\sqrt{\text{Hz}}$. For our sample, we then find $\sqrt{S_\epsilon^0} = 6.6 \times 10^{-7}\,\text{V}/\sqrt{\text{Hz}}$.

These noise estimates are used in Sec. S.3 C to calculate the gate fidelities we expect to reach theoretically, which we then compare to our experimental results.

## S.3. OPTIMAL PULSES

### A. Bloch sphere convention

Throughout this work, we use the convention that $J(\epsilon)$ coincides with the Bloch sphere's $y$-axis and $\Delta B_z$ with the $z$-axis.

If $J(\epsilon)$ would point along the $x$-axis of the Bloch sphere, our $\pi/2_x$ ($\pi/2_y$) gate would actually correspond to a $\pi/2$ rotation around the negative $y$-axis (positive $x$-axis). For ease of understanding, we thus apply a coordinate system transformation so that that $J(\epsilon)$ points along the $y$-axis. In this frame, the $\pi/2_x$ ($\pi/2_y$) gate rotates around the $x$-axis ($y$-axis) as expected.

### B. Numerical pulse optimization

The pulse optimization we perform for this work is similar to the one in supplementary Ref. 7. For completeness, we now provide a short summary and highlight any differences.

First, we characterize the step response of our electrical setup and measure $J_0$, $\epsilon_0$ and $\Delta B_z$ as described in Sec. S.2 A. We also determine the coherence of our qubit as described in Sec. S.2 B. Consequently, we use this information as a model for the numerical pulse optimization of piece-wise constant detuning pulses with $N_{\text{seg}}$ segments. Each pulse segment is 1 ns long, corresponding to the sampling rate of our AWG. In the following, $\epsilon_j$ with $j = 1 \ldots N_{\text{seg}}$ denotes the detuning in the $j^{\text{th}}$ segment. The actual control pulse arriving at the qubit is determined by applying a filter to the piece-wise constant pulse $\epsilon_j$ (see Sec. S.2 A). This is even more realistic than the procedure outlined in supplementary Ref. 7 where a purely exponential model was used to account for finite rise times.

We also choose slightly different bounds than supplementary Ref. 7 and constrain the detuning to $0.26\,\text{mV} \leq \delta \leq 4.00\,\text{mV}$. The upper bound of $\delta$ corresponds to the $(1, 1)$ charge regime with separated electrons. At this point $J \ll \Delta B_z$ is essentially turned off and $\epsilon$ is at the baseline $\epsilon_{\text{min}}$ mentioned in the main text. The lower bound was chosen to avoid the anticrossing of the singlet state with the $|\text{T}_+\rangle$ state during gate operation. This anticrossing occurs at large detunings $\epsilon$, typically at a distance $\delta \approx 0.22\,\text{mV}$ from the measurement point M. The crossing is also indicated in Fig. 1 and Fig. S.2. We avoid pulsing across this anticrossing as it would lead to a significant portion of the singlet state being converted to $|\text{T}_+\rangle$ and as such increase the gate leakage rate. For future experiments, it would be helpful to further examine the process driving leakage so that it can be captured and minimized directly in the numerical pulse optimization.

Furthermore the last 4 ns (5 ns) of each gate were set to $\epsilon_{\text{min}}$ (which corresponds to $\delta = 4.00\,\text{mV}$) for the 24 ns long gates in Fig. 2 (30 ns long gates in Fig. 3) to ensure that the pulse has decayed to $\epsilon_{\text{min}}$ before another gate is applied. If the decay is not perfect, transients from the previous gate will affect the next gate. Since such gate bleedthrough[8] causes additional errors which depend on the sequence of gates and not just the gates themselves, it is harder to detect and correct than purely gate-dependent errors. Thus, it is best to minimize gate transients whenever possible.

For the pulse optimization, explicitly time-dependent Hamiltonians $H(J(\epsilon(t)), \Delta B_z) = \frac{\hbar J(\epsilon(t))}{2}\sigma_x + \frac{\hbar \Delta B_z}{2}\sigma_z$ are approximated as piecewise constant on 0.2 ns intervals. This discretization greatly simplifies the calculation of $U(t, t_0) = \mathcal{T} \exp\left(-\frac{i}{\hbar}\int_{t_0}^{t} H(t')\,dt'\right)$ and incurs only small systematic errors on the order of $10^{-3}$ (in fidelity). These can be calibrated in experiments by using GAMBIT (Gate Adjustment by Iterative Tomography). Using this approximation, we can also calculate the effect of quasistatic noise in $\epsilon$ and $\Delta B_z$. All we have to do is to repeat the calculation several times using $H(J(\epsilon(t) + d\epsilon), \Delta B_z + d\Delta B_z)$, where $d\epsilon$ ($d\Delta B_z$) is sampled discretely from a Gaussian distribution with standard deviation $\sigma_\epsilon$ ($\sigma_{\Delta B_z}$). It is a little bit more involved to include fast noise with an arbitrary noise spectral density in a computationally efficient manner. We choose to use a first-order perturbative approach based on filter functions[9] which is fast enough for numerical optimization.

We then combine these methods with the Levenberg-Marquardt algorithm (LMA) to search for $\pi/2_x$ and $\pi/2_y$ pulses with maximal fidelity $\mathcal{F}$, taking systematic errors and the major decoherence sources into account. Further details regarding the exact implementation of the optimization are given in supplementary Ref. 7. An example of the resulting pulses $\epsilon_j^g, j = 1 \ldots N_{\text{seg}}$ for two gates $g = \pi/2_x$ and $g = \pi/2_y$ can be found in Fig. 2a.

### C. Fidelity estimation

Using the noise model described in Sec. S.2 B, we use Monte Carlo simulations as in supplementary Ref. 7 to determine the average gate fidelity of the gate set used in Fig. 3a. For hyperfine noise we use $\sigma_{\Delta B_z} = 2\pi \cdot 2.5\,\text{MHz}$. We find an average gate fidelity of 98.8 % which is in good agreement with the fidelity of $(98.5 \pm 0.1)$ % from randomized benchmarking, given that the charge noise model for the high frequencies relevant for nanosecond

TABLE S.1. **Theoretical infidelity contributions.** The different noise contributions to $\mathcal{I} = 1 - \mathcal{F}$ are obtained using Monte Carlo simulations (1000 time traces)[7] for the gates used in Fig. 3a. All charge noise below 1 MHz is included in $\mathcal{I}_{\epsilon,\mathrm{slow}}$, using noise strengths from Sec. S.2 B. Faster charge noise is taken into account in $\mathcal{I}_{\epsilon,\mathrm{fast}}$. The infidelity due to hyperfine noise, $\mathcal{I}_{\Delta B_z}$, is much smaller than the charge noise contributions. In the simulation, the gate was implemented perfectly as indicated by the low unitary infidelity, $\mathcal{I}_U$.

| | $\pi/2_x$ | $\pi/2_y$ |
|---|---|---|
| $\mathcal{I}_{\epsilon,\mathrm{fast}}$ | $6.4 \times 10^{-3}$ | $5.1 \times 10^{-3}$ |
| $\mathcal{I}_{\epsilon,\mathrm{slow}}$ | $5.3 \times 10^{-3}$ | $3.9 \times 10^{-3}$ |
| $\mathcal{I}_{\Delta B_z}$ | $1.6 \times 10^{-3}$ | $1.8 \times 10^{-3}$ |
| $\mathcal{I}_U$ | $6.3 \times 10^{-10}$ | $0.5 \times 10^{-10}$ |
| $\mathcal{I}$ | $1.4 \times 10^{-2}$ | $1.0 \times 10^{-2}$ |

gates is not known and was extrapolated. The noise contributions to the infidelity $\mathcal{I} = 1 - \mathcal{F}$ listed in Tab. S.1 indicate that charge noise is the dominant factor for decoherence.

To assess the potential for further improvement with the same noise characteristics, it is instructive to consider the effect of stretching or compressing one of our numerically optimized pulses in time. Doing so results in distinct scaling laws of the contributions to $\mathcal{I}$ from different noise types. For fast charge noise, the scaling law also depends on the spectral noise density $S_\epsilon(f) \propto 1/f^\beta$. When we change the total duration $T$ of a pulse and accordingly adjust $J(\epsilon)$ and $\Delta B_z$ so that the same unitary is still realized, we find

$$\mathcal{I}_{\epsilon,\mathrm{fast}} \propto T^{\beta-1}, \quad \text{(S.3)}$$

$$\mathcal{I}_{\epsilon,\mathrm{slow}} \sim \mathrm{const}, \quad \text{(S.4)}$$

$$\mathcal{I}_{\Delta B_z} \propto T^2, \quad \text{(S.5)}$$

assuming $\mathcal{I} \ll 1$. $\mathcal{I}_{\Delta B_z}$ increases with $T$ since $\Delta B_z$ decreases with $T$ while the standard deviation of $\Delta B_z$ remains the same. Thus, the error of the phase acquired due to $\Delta B_z$ increases with $T$. For slow charge noise we need to additionally consider $dJ/d\epsilon$ which decreases with $J$. Consequently, the standard deviation of $J(\epsilon)$ decreases with $T$ and $\mathcal{I}_{\epsilon,\mathrm{slow}}$ is approximately constant. For high-frequency charge noise the form of the noise spectrum given by the exponent $\beta$ needs to be taken into account since the frequency range most relevant for the gate changes with $1/T$. Using the filter function formalism[9], $\mathcal{I}_{\epsilon,\mathrm{fast}} \propto T^{\beta-1}$ can be derived.

Combining the noise contributions in Tab. S.1 with Eqs. (S.3-S.5) allows us to calculate which duration $T$ is optimal for our $\pi/2_x$ and $\pi/2_y$ gate. We find that the $\pi/2_x$ and $\pi/2_y$ gate could be improved by decreasing $T$ by 20 % and 30 %, respectively. However, doing so would only increase the gate fidelity by about $1 \times 10^{-4}$ ($3 \times 10^{-4}$). Thus, the original gates are already close to optimal and no further modification is needed.

## S.4. READOUT AND INITIALIZATION

### A. Pulses

The FID and SE experiments used for measuring hyperfine noise (see Sec. S.2 B) are performed with singlet initialization and readout.

For all other experiments, we prepare the state $|\uparrow\downarrow\rangle$ adiabatically. To this end, we first decrease $\epsilon$ quickly and diabatically jump over the S-T$_+$ transition to avoid mixing with the $|\mathrm{T}_+\rangle$ level. Then, we slowly ramp $\epsilon$ down to $\epsilon_{\mathrm{min}}$. In this way, $J(\epsilon)$ is turned off adiabatically since $J(\epsilon_{\mathrm{min}}) \ll \Delta B_z$. For readout, we slowly sweep $\epsilon$ from $\epsilon_{\mathrm{min}}$ up to a point before the S-T$_+$ transition. Then, we jump directly to the measurement point $\epsilon_{\mathrm{M}}$. Since we cross the S-T$_+$ transition diabatically we avoid mixing with the $|\mathrm{T}_+\rangle$ level. Since $J(\epsilon)$ is turned back on adiabatically we measure in the basis $\{|\uparrow\downarrow\rangle, |\downarrow\uparrow\rangle\}$.

### B. Data acquisition

Data is acquired in buffers with a duration of approximately 100 ms. Each buffer contains $\sim 20$ repetitions of $N \sim 1000$ pulse sequences, and we typically measure between 10 to 1000 buffers in order to ensure good averaging over the slowly decorrelating $\Delta B_z$. Every pulse sequence consists of an adiabatic initialization pulse to prepare $|\uparrow\downarrow\rangle$, qubit manipulation pulses and adiabatic readout, which maps singlet and triplet probabilities to $|\uparrow\downarrow\rangle$ and $|\downarrow\uparrow\rangle$ probabilities. In the following we refer to singlet probabilities $p(|0\rangle)$ whenever we mean the probability of measuring $|\uparrow\downarrow\rangle$.

After each buffer, polarization pulses[4] are applied to stabilize the hyperfine gradient $\Delta B_z$. Once in about $10^3$ measurements we also read out a completely mixed state and a triplet state as additional references. While the mixed state is prepared by rotating around various axes with different $J(\epsilon)$ for times on the order of a µs, much longer than the coherence time $T_2^*$ of the qubit, the triplet state is prepared by precession of a singlet state in the stabilized hyperfine field $\Delta B_z$.

We discriminate between singlet and triplet states by Pauli spin blockade. Using spin to charge conversion[10], the resistance of an adjacent sensing dot depends on the spin state and can be determined by RF-reflectometry[11]. In this manner, we obtain different readout voltages for singlet and triplets states, $U_{|\mathrm{S}\rangle}$ and $U_{|\mathrm{T}_0\rangle}$, but cannot distinguish between $|\mathrm{T}_0\rangle$ and the triplet states $|\mathrm{T}_\pm\rangle$.

We only switch the RF readout power on during measurements while leaving it off during manipulation. The timing of this switching is chosen carefully to minimize the influence of transients on the measured voltages.

The voltages measured in a buffer, which contains about 20 repetitions of a sequence of $N \sim 1000$ pulses, are processed in two ways:

1. All measured voltages are binned, irrespective of

the pulse sequence or repetition they are associated with, to obtain histograms of the readout values.

2. Measured voltages corresponding to repetitions of the same pulse sequence are averaged, yielding $N$ averaged voltages $U$.

Since data requirements differ between the various experiments, details about further data processing and our readout calibration are given in separate sections, specifically in Sec. S.5 A, Sec. S.5 B and Sec. S.5 C.

### C. Data postselection

For all measurements, we automatically detect switching events due to charge traps and remove the affected data points.

Furthermore we discard data where dynamic nuclear polarization (DNP) was not stable and deviated by more than $\pm\sigma_{\Delta B_z} \approx \pm 2\pi \cdot 2.5\,\mathrm{MHz}$ from the set point of $\Delta B_z$ at about $2\pi \cdot 61.6\,\mathrm{MHz}$.

While $\Delta B_z$ postselection is performed to remove datasets with unstable DNP, this procedure might also lead to increased gate fidelities. However, due to the relatively weak influence of hyperfine noise on gate performance (see Tab. S.1) we do not expect this effect to be significant.

### D. Mapping state preparation to measurement errors

In this section, we argue that state preparation errors can be mapped to measurement errors. Hence, we only need to consider the latter in following discussions.

By definition, state preparation does not suffer from systematic errors as it defines the computational basis states $|0\rangle$ and $|1\rangle$. However, the purity of the initial state can be finite due to stochastic errors from incomplete relaxation to the ground state[12] or from a combination of imperfect adiabaticity and dephasing. As a check, we prepare $|\uparrow\downarrow\rangle$, let it evolve for varying times (between 0 ns and 24 ns in 1 ns increments) and read out along different axes than $z$ using diabatic pulses before the adiabatic readout. Since the resulting readout voltages do not show sinusoidal oscillations, we conclude that imperfect adiabaticity is not a problem for our initialization (dephasing should occur on a timescale of $T_2^* \geq 80\,\mathrm{ns}$).

Since we use the same sweep speed for the adiabatic ramps used for state initialization and readout, our readout should be along the same axis as the state preparation. We check whether this assumption is justified by preparing different initial states than $|\uparrow\downarrow\rangle$ (using diabatic pulses after the adiabatic initialization) and letting them evolve in the hyperfine field at $J(\epsilon_{\mathrm{min}})$ for varying times (between 0 ns and 24 ns in 1 ns increments) before adiabatic readout. The resulting readout voltages do not show sinusoidal oscillations. Thus, we can deduce that readout and initialization axes coincide with the rotation axis at $J(\epsilon_{\mathrm{min}})$ since in neither case oscillations could be observed. Thus, readout and initialization are performed along the same axis (up to measurement noise, which could have been larger than a small sinusoidal signal). Note that readout and initialization can still suffer from different stochastic errors.

Since it is impossible to discriminate stochastic state preparation errors from readout errors, the state preparation can be treated as perfect and all state preparation errors can be mapped to our adiabatic measurement[12]. Adiabatic state preparation and adiabatic measurement are performed along the same axis as explained above.

## S.5. READOUT CALIBRATION

In this section, we discuss how readout signals are processed for the different type of data sets presented.

### A. Self-consistent state tomography

For self-consistent state tomography (see Sec. S.7 A and Fig. 2d), we convert measured voltages to singlet probabilities $p(|0\rangle)$ by fitting the bimodal histogram[13] obtained from binning the measurement data (see Sec. S.4 B).

In contrast to supplementary Ref. 13, we observe excitation from $|\mathrm{S}\rangle$ to $|\mathrm{T}_0\rangle$ as well as relaxation from $|\mathrm{T}_0\rangle$ to $|\mathrm{S}\rangle$. Since the standard model[13] does not fit our data well, we extend it by including an excitation rate $e$ from $|\mathrm{S}\rangle$ to $|\mathrm{T}_0\rangle$ in addition to the relaxation rate $r$. In separate experiments we measure $T_1$ decays in the $(2, 0)$ charge region where readout is performed. From this data, we determine $T_1$ and the steady state voltage $V_{\mathrm{SS}}$ to which states decay after long times in the $(2, 0)$ charge region. $T_1$ and $V_{\mathrm{SS}}$ are then used as additional fixed parameters in the fit of the histograms. The resulting fits typically look like the one in Fig. S.3. $U_{|\mathrm{S}\rangle}$ and $U_{|\mathrm{T}_0\rangle}$ can then be calculated from the fit parameters and correspond to singlet probabilities of $p(|0\rangle) = 1$ and $p(|0\rangle) = 0$.

We can now convert the averaged voltages to singlet probabilities $p(|0\rangle) \in [0, 1]$ using a linear transformation $p(|0\rangle) = \frac{1}{2}\langle\sigma_z\rangle + \frac{1}{2} = \frac{c}{2}(U + s) + \frac{1}{2}$ with coefficients $c$ and $s$ obtained from the fit. Inaccuracies from fitting of the single shot histogram do not affect the tomography results as self-consistent state tomography is insensitive to state preparation and measurement (SPAM) errors.

### B. Benchmarking

For our benchmarking experiments (see Sec. S.7 B and Fig. 3) we perform a similar calibration as described in the previous section for self-consistent state tomography (Sec. S.5 A).

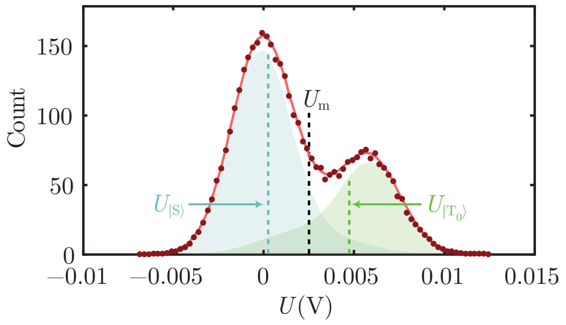


FIG. S.3. **Readout calibration.** We fit a readout model (light red)[13] to the binned readout voltages of an entire buffer (dark red). The fitted underlying distributions of singlet and triplet voltages are shown in blue and green, respectively. The 50th percentile of each distribution is indicated by a dashed line. Extending previous work[13], relaxation (from triplet to singlet) and excitation (from singlet to triplet) are taken into account. The voltages corresponding to singlet $U_{|\mathrm{S}\rangle}$, triplet $U_{|\mathrm{T}_0\rangle}$ and the completely mixed state $U_\mathrm{M}$ are indicated.

In addition, we now consider that long gate sequences create a significant $|\mathrm{T}_+\rangle$ population. For the readout calibration we have so far neglected that other states than $|\mathrm{T}_0\rangle$ and $|\mathrm{S}\rangle$ might be populated. We have attempted to include $|\mathrm{T}_+\rangle$ explicitly in the fit model but found that this introduces too many additional parameters. To circumvent systematic shifts of the fitted $U_{|\mathrm{S}\rangle}$ and $U_{|\mathrm{T}_0\rangle}$ and achieve an approximate calibration, we include an additional constraint in the histogram fit which enforces that the mixed state reference voltage $U_\mathrm{M}$ always corresponds to $p(|0\rangle) = 0.5$. While we have not quantitatively analyzed the error from this approximate procedure, we suspect that the suboptimal contrast in Fig. 3 might be related.

As RB and all other benchmarking experiments performed in this work are insensitive to SPAM errors, our readout calibration does not need to be especially accurate or precise. Specifically, the suboptimal contrast does not affect any figures of merit reported in this work.

### C. GAMBIT

For optimization with GAMBIT, the averaged voltages $U_i$ corresponding to the error syndromes $S_i$ (as defined in Tab. I) do not need to be explicitly converted to singlet probabilities $p(|0\rangle)$ or $\langle\sigma_z\rangle$ as in the previous two sections (Sec. S.5 A and Sec. S.5 B). Instead, $\tilde{U}_i = |U_i - U_{\mathrm{M/T}}|$ can be optimized without further calibration. In this expression $U_{\mathrm{M/T}}$ corresponds to $U_\mathrm{M}$ if $i = 1\ldots6$, otherwise the voltage $U_\mathrm{T}$ of the reference $|\mathrm{T}_0\rangle$ state is used. The reference triplet state $|\mathrm{T}_0\rangle$ is subject to decoherence because it is prepared by letting $|\mathrm{S}\rangle$ evolve in the hyperfine field at $J(\epsilon_{\min}) \ll \Delta B_z$. $U_\mathrm{T}$ is obtained by correcting the actual measurement result $U'_\mathrm{T}$ for the approximate loss in contrast of the triplet preparation using the transformation $U_\mathrm{T} = U'_\mathrm{T} + b(U'_\mathrm{T} - U_\mathrm{M})$ with $b \sim 10^{-2}$ chosen according to $T_2^*$ measurements. The exact choice of $b$ is not crucially important as long as reductions in the decoherence of the gate set result in a reduction of $S_7$ and $S_8$. Furthermore, $S_7$ and $S_8$ should be of comparable magnitude as the other syndromes for optimal convergence. This can be achieved by choosing appropriate weights $w_7$ and $w_8$ in Eq. (S.15).

It is helpful to compensate fluctuations of the measurement contrast with the aid of histograms to speed up convergence. With $c$ and $s$ defined as in Sec. S.5 A this yields

$$\begin{aligned}\tilde{S}_i &= c\tilde{U}_i &\text{(S.6)}\\ &= |c(U_i + s) - c(U_{\mathrm{M/T}} + s)| &\text{(S.7)}\\ &= |S_i - S_{\mathrm{M/T}}|, &\text{(S.8)}\end{aligned}$$

which is the same relation as given in the main text.

## S.6. GAMBIT

### A. Error syndromes

The gate sequences from Tab. I used to extract the error syndromes are modified versions of the previously published bootstrap tomography[14]. GAMBIT uses the information obtained from the error syndromes in a specific manner explained in Sec. S.6 C. As described in the methods section of the paper and in Sec. S.4 A, we adiabatically prepare $|\uparrow\downarrow\rangle$ before applying any of the gate sequences from Tab. I or Tab. S.2. At the end of each gate sequence, we read out adiabatically, allowing us to discriminate between $|\uparrow\downarrow\rangle$ and $|\downarrow\uparrow\rangle$.

Possible errors include decoherence and systematic errors, which can be categorized as over-rotation and off-axis errors. We use the same parameterization for systematic errors as in supplementary Refs. 7 and 14 and denote the rotation-angle error of the $\pi/2_x$ ($\pi/2_y$) gate by $2\phi$ ($2\chi$) while axis-errors are described by $n_y, n_z$ ($v_x, v_z$). Using this notation, the unitary operator of the erroneous $\pi/2_x$ gate can be written as

$$U_x = \exp\left[-i(\boldsymbol{n}\cdot\boldsymbol{\sigma})(\pi/2 + 2\phi)/2\right] \tag{S.9}$$

$$\text{with } \boldsymbol{n} = \left(\sqrt{1 - n_y^2 - n_z^2},\ n_y,\ n_z\right)^\top. \tag{S.10}$$

Likewise, the unitary operator of the erroneous $\pi/2_y$ gate is given by

$$U_y = \exp\left[-i(\boldsymbol{v}\cdot\boldsymbol{\sigma})(\pi/2 + 2\chi)/2\right] \tag{S.11}$$

$$\text{with } \boldsymbol{v} = \left(v_x,\ \sqrt{1 - v_x^2 - v_z^2},\ v_z\right)^\top. \tag{S.12}$$

The first six sequences are sufficient to extract all systematic errors, and we introduce two additional sequences to explicitly probe for decoherence. When the systematic errors of the gate set are small, the amplification sequences in Tab. S.2 are used instead of Tab. I, resulting in three-fold amplification of the rotation-angle errors

$2\phi$ and $2\chi$ and the axis-errors $n_y$ and $v_x$. It is possible to achieve higher amplification by repeating the gate sequences multiple times but this also increases the overall decoherence. Since decoherence can lead to systematic shifts of the syndromes, the extracted error signature becomes less reliable for long gate sequences.

### B. Insensitivity to measurement errors

In this section we discuss GAMBIT's insensitivity to SPAM errors. As pointed out in Sec. S.4 D, all adiabatic state preparation errors can be mapped to the adiabatic measurement. Thus, we can focus solely on measurement errors in this section. Furthermore, we have discussed in Sec. S.4 D that the state preparation axis and measurement axis align in our system. Since GAMBIT works with only one readout axis and does not require precalibrated gates, the relevant readout errors can be captured by a reduction in contrast $\delta_c$ ($0 \leq \delta_c \leq 1$) and a shift $\delta_s$ ($-1 \leq \delta_s \leq 1$) of the measurement results.

These parameters capture that measuring the error syndrome $S_i$ will generally not result in the correct voltage $U_i$ but instead yield $U_i' = \delta_c(U_i + \delta_s)$. Note that some further constraints on $\delta_c$ and $\delta_s$ are needed to ensure that the measurement stays physical. As described in Sec. S.5 C, GAMBIT optimizes

$$\tilde{S}_i = |c(\delta_c U_i + \delta_c\delta_s + s) - c(\delta_c U_\mathrm{M} + \delta_c\delta_s + s)| \quad \text{(S.13)}$$
$$= |c\delta_c(U_i - U_\mathrm{M})| \quad \text{(S.14)}$$

so that shifts $\delta_s$ are of no consequence.

Changes in the measurement contrast $\delta_c$ will lead to slower convergence as discussed in Sec. S.6 D. However, the feedback loop should still converge to the same target as $|c\delta_c(U_i - U_\mathrm{M})|$ is always zero for a perfect gate set, irrespective of $\delta_c$. As pointed out in Sec. S.5 C, histograms of the measured voltages can be used to determine $c$ so that $c\delta_c$ is approximately constant. Hence, GAMBIT can be made insensitive to fluctuations $\delta_c$ as long as $c\delta_c$ does not change significantly between GAMBIT iterations.

TABLE S.2. **Amplifying gate sequences.** To first order, the outcome of the measurement $\mathrm{Tr}(\sigma_z U_i |0\rangle\langle 0| U_i^\dagger) = S_i$ depends linearly on the gates' rotation-angle errors $2\phi$ ($2\chi$), the axis-errors $n_y, n_z$ ($v_x, v_z$) and decoherence $d_x$ ($d_y$) of the $\pi/2_x$-gate ($\pi/2_y$-gate). Parametrization defined in the text and in supplementary Refs. 7 and 14. Here, the amplification sequences used for GAMBIT are shown.

| Sequences $U_i$ | Parametrization | $S_i$ |
|---|---|---|
| $(\pi/2_x)^3$ | $6\phi =$ | $S_1$ |
| $(\pi/2_y)^3$ | $6\chi =$ | $S_2$ |
| $(\pi/2_y \circ \pi/2_x)^4$ | $-2\chi - 3n_y - n_z - 2\phi - 3v_x - v_z =$ | $S_3$ |
| $(\pi/2_x) \circ (\pi/2_y)$ | $-n_y + n_z - v_x + v_z =$ | $S_4$ |
| $(\pi/2_x)^3 \circ (\pi/2_y)$ | $n_y + n_z + v_x - v_z =$ | $S_5$ |
| $(\pi/2_x) \circ (\pi/2_y)^3$ | $n_y - n_z + v_x + v_z =$ | $S_6$ |
| $(\pi/2_x)^2$ | $d_x =$ | $S_7$ |
| $(\pi/2_y)^2$ | $d_y =$ | $S_8$ |

### C. Feedback loop

Before the feedback loop is started, we perform a scaling analysis to compensate shifts in $J(\epsilon)$. To this end, we independently scale the $\epsilon$ pulses of both gates. Specifically, we scale the amplitude minus the baseline, $\epsilon_j^g - \epsilon_\mathrm{min}$, by $\pm 20\%$ in increments of $4\,\%$ and measure all 8 error syndromes for each scale factor. We start the iteration with the best scale factor chosen separately for each gate.

For the iterative control loop we use the Levenberg-Marquardt Algorithm (LMA), which requires derivatives of the objective function to compute an update. Throughout this work, the LMA iteratively solves the problem

$$\min_{\epsilon_j^g} \left| \left( \tilde{\mathbf{S}}_{\mathbf{1-6}}(\epsilon_j^g),\ w_7\tilde{S}_7(\epsilon_j^g),\ w_8\tilde{S}_8(\epsilon_j^g) \right) \right|^2, \quad \text{(S.15)}$$

where $\tilde{\mathbf{S}}_{\mathbf{1-6}}$ is a six-component row vector consisting of the first six error syndromes $\tilde{S}_i, i = 1\dots 6$ (see Tab. I and Sec. S.5 C). This minimization problem is a slightly modified version of Eq. (2) from supplementary Ref. 7. The weights $w_7$ and $w_8$ should be chosen such that the vector components do not differ by orders of magnitude. Here, they were chosen heuristically as 0.5 so that the last two vector components are approximately proportional to the decoherence of a single gate ($\tilde{S}_7$ and $\tilde{S}_8$ are obtained by applying $\pi/2_x$ and $\pi/2_y$ twice, respectively).

We use the LMA because we found in simulations that derivative free methods such as the Nelder-Mead algorithm (NMA) typically take at least an order of magnitude more iterations than the LMA to converge well. This of course only holds true as long as derivatives can be reliably measured. Minimizing the number of iterations is important as pulse updates on our arbitrary waveform generator (AWG) and reference measurements take about 2 min during which we cannot acquire new data. On the other hand we can perform on the order of $10^5$ measurements per second once pulses have been uploaded to the AWG. Consequently, we would like to minimize the number of iterations rather than the number of measurements.

We estimate the derivatives required for the LMA from measurement data using forward finite differences with a fixed step size. It is important to choose a finite difference step size which is large enough so that the numerical derivatives are not dominated by measurement noise. However, the estimation error becomes larger for large step sizes. The optimum step size depends on the curvature and magnitude of the objective function. Since curvature and magnitude depend on the point in parameter space and are not generally known, we simulate GAMBIT, and find a step size $h = 0.2\epsilon_0 \dots 0.3\epsilon_0$ to be optimal for a noise level of $1 \times 10^{-2}$ of the measured singlet

probability $p(|0\rangle)$. These values also work well in our experimental setup.

Overall, one iteration takes about 10 min. This includes the time needed for measuring the finite differences, pulse updates on the AWG and post-processing of the data on a standard desktop computer.

### D. Convergence

Not considering large charge rearrangements, the speed of convergence is similar to what we expect from simulations[7], where SPAM errors were completely disregarded. As mentioned in Sec. S.6 B, GAMBIT should be insensitive to slow shifts of the readout voltages. But slow changes in the measurement contrast $\delta_c$ will affect $\tilde{S}_i = |c\delta_c(U_i - U_\mathrm{M})|$ if not compensated by a different choice of $c$ so that $c\delta_c$ remains approximately constant. If this is the case, derivatives $d\tilde{S}_i/d\epsilon_j^g$ cannot be reliably measured and suboptimal updates of the pulse parameters $\epsilon_j^g$ will be performed. Since the speed of convergence is similar to the simulations, choosing $c$ from histogram fits seems to work well.

As in the simulations[7], convergence stops when the noise floor has been reached. For our experiments, we measured enough data points for each different gate sequence so that a noise level of approximately $10^{-2}$ of $\langle\sigma_z\rangle = 2p(|0\rangle) - 1$ is obtained. With this noise level we find that convergence typically stops when the signals $\tilde{S}_i$ are on the order of $10^{-1}$. However, the simulations converge to lower syndromes $\tilde{S}_i \approx 3\times 10^{-2}$ for the same noise level[7]. This discrepancy could arise from specific forms of gate related decoherence which affects $\tilde{S}_i$. Additionally, charge drifts in our noisy sample could lead to changes in the detuning $\epsilon$ (which is equivalent to a change in $J_0$) and hence slowly shift the target during the optimization.

Furthermore, relatively frequent charge rearrangements complicate matters. These typically lead to large changes in $J(\epsilon)$ and dramatically affect which pulse parameters $\epsilon_j^g$ are optimal. If charge rearrangements occur within an optimization run, we proceed as follows: Initially, we wait for the dot to return to the previous configuration and discard the data recorded in the wrong dot configuration. While there seem to be less than 10 different dot configurations which can be explained by several nearby charge traps, it can take a long time (up to days) for the dot to return. Thus, we manually tune the dot back to a working configuration if the original configuration has not been restored after a short while (~ hours). As gate performance is very sensitive to the exact functional form of $J(\epsilon)$, manual tuning of the dot typically leads to a deterioration of gate fidelity. Depending on the amount of tuning required, we can either continue with the optimization (see for example Fig. 2e) or need to start from the beginning.

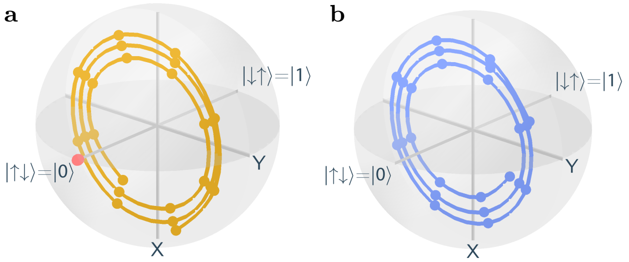


FIG. S.4. **Self-consistent state tomography.** FID experiments at $J = 0$. The states indicated by dots are reconstructed from an overcomplete set of information, using six different measurements. **a** The state $|0\rangle$ shown by the red dots is an eigenstate and does not evolve. This is different for the initial state of the other FID experiment and the state shown in blue in panel **b**.

## S.7. GATE BENCHMARKS

### A. Self-consistent state tomography

Following supplementary Ref. 12, we calibrate the self-consistent state tomography using five FID experiments for five different initial states with the exchange interaction switched off ($\epsilon = \epsilon_\mathrm{min}$). For each free evolution, multiple points are read out along six different measurement axes. This overcomplete set allows us to determine the five initial states and six measurement operators from a self-consistent fit. Following the argument in Sec. S.4 D, we assume for the fit that the axes of adiabatic state preparation and measurement align, and that all initialization errors can be mapped to the measurement.

Any unknown state is consequently read out using the six measurement operators known from the calibration. Since this again results in overcomplete information as only three linearly independent measurement operators would be needed, the unknown state is determined as the best fit (in the least-squares sense) to the overcomplete information. The states for different evolution times of FID experiments reconstructed in this way are shown in Fig. S.4, showing good agreement with the expected trajectories.

The gate trajectories in Fig. 2d are obtained in the same way. The gate operation is stopped in increments of 1 ns and the resulting final state read out. There is a small caveat however. The state tomography was calibrated for readout pulses which start at $\epsilon = \epsilon_\mathrm{min}$. While the gate operation returns to $\epsilon_\mathrm{min}$ in the end, intermediate points may be at $\epsilon > \epsilon_\mathrm{min}$. Due to finite bandwidth effects, the measurement operator will then vary with $\epsilon$ and might be different than in the calibration. Thus, readout is only reliable if the previous operation has already reached $\epsilon_\mathrm{min}$ before the state is read out (including finite rise times). Such concatenation errors contribute to the deviations between the trajectories shown in Fig. 2c

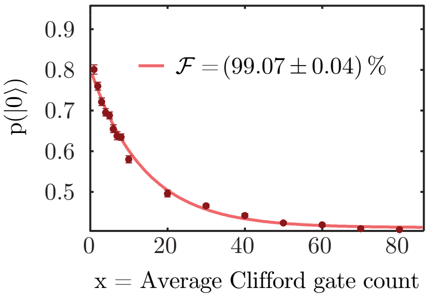


FIG. S.5. **Standard randomized benchmarking.** The data points shown in dark red are the same as in Fig. 3a. The light red curve shows a standard randomized benchmarking fit which yields a gate fidelity of $(99.07 \pm 0.04)\,\%$. When leakage is taken into account, a lower gate fidelity of $(98.5 \pm 0.1)\,\%$ is extracted (see Fig. 3a).

and Fig. 2d when the exchange interaction is switched on.

### B. Randomized benchmarking and leakage

For randomized benchmarking (RB), we compose Clifford operations from the primitive gate set according to Tab. S.3, resulting in an average of 3.75 primitive gates per Clifford. This procedure is commonly used in other works which use RB for gate characterization, e.g. by supplementary Ref. 15. In addition to the benchmarking experiments mentioned in the main text, we also apply standard randomized benchmarking (RB) without taking leakage into account.

Fig. S.5 shows a fit applied to the data shown in red in Fig. 3a, yielding a gate fidelity of $(99.07 \pm 0.04)\,\%$. The standard fit model[16] with $x$ denoting the number of applied Clifford gates (without the inversion gate)

$$p_{\mathrm{RB}}(|0\rangle)(x) = A \cdot (1-2r)^x + B \qquad \text{(S.16)}$$

yields the fit coefficients shown in the first column of Tab. S.4.

Since this fit model does not explain why the signal decays below $p(|0\rangle) = 0.5$, we combine it with a recently developed modified leakage randomized benchmarking (LRB) protocol[17] which omits the last Clifford gate from each RB sequence, resulting in the data shown in blue in Fig. 3a. We then simultaneously fit the equations

$$p_{\mathrm{RB}}(|0\rangle)(x) = A \cdot (1-2r)^x + B \cdot (1-l)^x + C \qquad \text{(S.17)}$$

$$p_{\mathrm{LRB}}(|0\rangle)(x) = D \cdot (1-l)^{x-1} + E \qquad \text{(S.18)}$$

to the red and blue data set, respectively. This yields the fit coefficients shown in the second column of Tab. S.4 from which the average fidelity $(98.5 \pm 0.1)\,\%$ and leakage rate $(0.4 \pm 0.1)\,\%$ for the primitive gate set from Fig. 3a are extracted. The leakage rate $l$ reported here is the sum $l = l^{c\to l} + l^{l\to c}$, where $l^{c\to l}$ denotes leakage out of the computational subspace into the leakage subspace and $l^{l\to c}$ leakage from the leakage subspace to the computational subspace[17]. While the origin of leakage is not firmly established, we conjecture that leakage into $|\mathrm{T}_+\rangle$ is dominant since our gate pulses approach the S-$\mathrm{T}_+$ transition. The presence of a single leakage level is supported by the fact that $p(|0\rangle)$ roughly approaches $1/3$ ($C = 0.3557$). Since $p(|0\rangle)$ corresponds to a singlet probability $p(|\mathrm{S}\rangle)$ due to the adiabatic readout (see Sec. S.4 A), the asymptote is consistent with $|\mathrm{S}\rangle$, $|\mathrm{T}_0\rangle$ and $|\mathrm{T}_+\rangle$ being occupied with the same probability when $x \to \infty$. While $C$ is sensitive to SPAM errors, it clearly deviates from 0.5. Thus, leakage represents the most plausible explanation for the observed second decay rate, irrespective of SPAM errors.

In addition to leakage, another caveat in RB are gate-dependent errors which are likely to be present here since the Clifford operations are generated from a limited primitive gate set. If we add a term for gate-dependent errors of the form $F(x-1)(1-2r)^{x-2}$ in Eq. (S.17)[16,18], the other fit coefficients change only slightly while $F$ turns out to be insignificantly different from zero. However, the errors on $r$, $A$ and $F$ are rather large (on the order of 10). This indicates that the fit cannot distinguish between the added term and $A \cdot (1-2r)^x$. The fit is therefore not conclusive. However, numerical simulations suggest that even in the case of gate-dependent errors or $1/f$-noise, benchmarking provides a "better than a factor-of-2 estimate of the average error rate" (p.11 of supplementary

TABLE S.3. **Clifford operations**. Sequences of primitive gates used to perform Clifford operations. $\bar{x}, \bar{y}$ and $\bar{z}$ denote the negative $x$-, $y$- and $z$-axis, respectively.

| Primitive gates | Clifford gates |
|---|---|
| $(\pi/2_y)^4$ | $(\mathbb{1})$ |
| $(\pi/2_x)^2$ | $(\pi_x)$ |
| $(\pi/2_y)^2$ | $(\pi_y)$ |
| $(\pi/2_x)^2 \circ (\pi/2_y)^2$ | $(\pi_z)$ |
| $(\pi/2_y) \circ (\pi/2_x)$ | $(\pi/2_y) \circ (\pi/2_x)$ |
| $(\pi/2_y)^3 \circ (\pi/2_x)$ | $(\pi/2_{\bar{y}}) \circ (\pi/2_x)$ |
| $(\pi/2_y) \circ (\pi/2_x)^3$ | $(\pi/2_y) \circ (\pi/2_{\bar{x}})$ |
| $(\pi/2_y)^3 \circ (\pi/2_x)^3$ | $(\pi/2_{\bar{y}}) \circ (\pi/2_{\bar{x}})$ |
| $(\pi/2_x) \circ (\pi/2_y)$ | $(\pi/2_x) \circ (\pi/2_y)$ |
| $(\pi/2_x)^3 \circ (\pi/2_y)$ | $(\pi/2_{\bar{x}}) \circ (\pi/2_y)$ |
| $(\pi/2_x) \circ (\pi/2_y)^3$ | $(\pi/2_{\bar{y}}) \circ (\pi/2_x)$ |
| $(\pi/2_x)^3 \circ (\pi/2_y)^3$ | $(\pi/2_{\bar{x}}) \circ (\pi/2_{\bar{y}})$ |
| $(\pi/2_x)$ | $(\pi/2_x)$ |
| $(\pi/2_x)^3$ | $(\pi/2_{\bar{x}})$ |
| $(\pi/2_y)$ | $(\pi/2_y)$ |
| $(\pi/2_y)^3$ | $(\pi/2_{\bar{y}})$ |
| $(\pi/2_x)^3 \circ (\pi/2_y)^3 \circ (\pi/2_x)$ | $(\pi/2_z)$ |
| $(\pi/2_x) \circ (\pi/2_y)^3 \circ (\pi/2_x)^3$ | $(\pi/2_{\bar{z}})$ |
| $(\pi/2_y) \circ (\pi/2_x)^2$ | $(\pi/2_y) \circ (\pi_x)$ |
| $(\pi/2_y)^3 \circ (\pi/2_x)^2$ | $(\pi/2_{\bar{y}}) \circ (\pi_x)$ |
| $(\pi/2_x) \circ (\pi/2_y)^2$ | $(\pi/2_x) \circ (\pi_y)$ |
| $(\pi/2_x)^3 \circ (\pi/2_y)^2$ | $(\pi/2_{\bar{x}}) \circ (\pi_y)$ |
| $(\pi/2_x) \circ (\pi/2_y) \circ (\pi/2_x)$ | $(\pi/2_x) \circ (\pi/2_y) \circ (\pi/2_x)$ |
| $(\pi/2_x) \circ (\pi/2_y)^3 \circ (\pi/2_x)$ | $(\pi/2_x) \circ (\pi/2_{\bar{y}}) \circ (\pi/2_x)$ |

TABLE S.4. **Randomized benchmarking fits.** Fit coefficients (with statistical errors) of different models fitted to our randomized benchmarking experiments.

| | Eq. (S.16) | Eq. (S.17-S.18) |
|---|---|---|
| $l$ | | $0.0154 \pm 0.0045$ |
| $r$ | $0.0349 \pm 0.0015$ | $0.0559 \pm 0.0052$ |
| $A$ | $0.3902 \pm 0.0065$ | $0.2983 \pm 0.0182$ |
| $B$ | $0.4125 \pm 0.0023$ | $0.1634 \pm 0.0179$ |
| $C$ | | $0.3557 \pm 0.0199$ |
| $D$ | | $0.1408 \pm 0.0169$ |
| $E$ | | $0.3553 \pm 0.0208$ |
| $\chi^2/dof$ | 2.2 | 0.9 |
| $\mathcal{F}$ | $0.9907 \pm 0.0004$ | $0.9851 \pm 0.0014$ |
| $\mathcal{L}$ | | $0.0041 \pm 0.0012$ |

Ref. 19). Thus, gate-dependent errors should not significantly influence our fidelity estimate.

Similar to RB, the derivation of the fit model for the leakage protocol assumes gate-independent noise. However, numerical simulations suggest that the protocol is robust even if gate-dependent noise is present[17]. Furthermore, the gate operations are required to form a unitary 1-design on the leakage space together with random $\pm$ phases between leakage and code level[17]. Since we do not have control over the leakage space and cannot read it out separately, this is hard to check for our nontrivial gate operations.

While we cannot check whether all formal prerequisites of the leakage protocol are satisfied, the exponential model fits the data well in the limit of long gate sequences so that the extracted rate itself is reliable. Furthermore, decoherence in the code space is nearly complete for gate counts greater than 200 so that leakage is the only physical process driving the slow decay. Since the omitted correction gate corresponds on average to an intentional inversion and only leaked states would not be driven to $p(|0\rangle) = 0.5$, it seems plausible that this rate is proportional to the actual leakage rate. We conclude that the fitted rate should therefore give a good indication of the actual leakage rate.

## C. Error amplification

To separate systematic errors from decoherence, we measure repetitions of $\pi/2_x$, $\pi/2_y$ and $\pi/2_x \circ \pi/2_y$. These sequences amplify over-rotation and axis errors, and typically result in data as shown in Fig. 3b. We fit this data using the parameters of two unitary operations given by rotation axis times rotation angle $\theta \cdot \vec{n}$, the probabilities $p_{\mathrm{depol}}$ of an added depolarizing channel, and separate leakage rates $\mathcal{L}$ for each of the two gates. We do not model the whole leakage space, but rather include leakage phenomenologically by subtracting a fraction $p(|0\rangle) \rightarrow (1-\mathcal{L})p(|0\rangle)$ with each applied gate since we are more interested in systematic effects rather than extracting a meaningful leakage rate. Thus, this approach should be sufficient to capture most of the effect of leakage, which will be small in the limit of short gate sequences anyway. All fit parameters are given in Tab. S.5. The systematic fidelity $\mathcal{F}_{\mathrm{sys}}$ is calculated by removing the depolarizing channel and leakage from the gates so that only systematic errors remain.

TABLE S.5. **Systematic errors**. Fit parameters of the fit in Fig. 3b which is used primarily to extract systematic errors of the gate set.

| | $\pi/2_x$ | $\pi/2_y$ |
|---|---|---|
| $\theta \cdot n_x$ | 1.5359 | 0.1461 |
| $\theta \cdot n_y$ | 0 | 1.4934 |
| $\theta \cdot n_z$ | $-0.2281$ | 0.1614 |
| $p_{\mathrm{depol}}$ | 0.0624 | 0.0647 |
| $\mathcal{L}$ | 0.0051 | 0.0021 |
| $\mathcal{F}_{\mathrm{sys}}$ | 0.9928 | 0.9926 |
| $\mathcal{F}$ | 0.9620 | 0.9608 |

Since our simplified decoherence model does not explain the observed behavior for a gate count larger than 12, and we are mainly interested in systematic errors, only the first 12 data points are fitted (solid light blue line in Fig. 3b). Fitting only data points not severely affected by decoherence should allow for a more reliable determination of the systematic errors because specific forms of decoherence can produce a behavior similar to systematic errors in these experiments. We are able to fit several periods of the oscillatory signal in the upper two panels of Fig. 3b and thus expect that the extracted rotation angles are accurate. Since the first 12 data points in the lower panel correspond only to about 1.5 periods, the extracted axes should be less accurate than the rotation angles.

The fit yields over-rotation errors of 1.5° and −3.5° and an angle between both rotation axes of 85.4°. The non-amplifyable angles with the $z$-axis are determined to be 98.4° and 83.9°. Overall, these deviations correspond to $\mathcal{F}_{\mathrm{sys}} = 99.3\,\%$, excluding decoherence. As RB yields $\mathcal{F} = (98.1 \pm 0.2)\,\%$ for this gate set, we conclude that decoherence and systematic errors contribute roughly equally. It is noticeable that while the leakage rate matches the one extracted in Fig. 3a for different gates, $\mathcal{F}$ differs from the RB result by about 2 percentage points. This is likely due to the simplified decoherence model, as otherwise the data points at higher gate counts would also be fitted well. In reality, decoherence can not be explained by a simple depolarizing channel due to the significant amounts of slow noise present. While Markovian depolarization would produce exponential ($T_2$-like) decay laws, non-Markovian errors will lead to a quadratic ($T_2^*$-like) decay arising from constructive interference or repeated errors. In the non-Markovian case, the infidelity corresponds to the initial decay so that fitting a Markovian model, as we do here, would overestimate the infidelity.

[1] Botzem, T. *et al.* Quadrupolar and anisotropy effects on dephasing in two-electron spin qubits in GaAs. *Nature Communications* **7**, 11170 (2016).

[2] Shulman, M. D. *et al.* Demonstration of entanglement of electrostatically coupled singlet-triplet qubits. *Science* **336**, 202–205 (2012).

[3] Dial, O. E. *et al.* Charge noise spectroscopy using coherent exchange oscillations in a singlet-triplet qubit. *Physical Review Letters* **110**, 146804 (2013).

[4] Bluhm, H., Foletti, S., Mahalu, D., Umansky, V. & Yacoby, A. Enhancing the Coherence of a Spin Qubit by Operating it as a Feedback Loop That Controls its Nuclear Spin Bath. *Physical Review Letters* **105**, 216803 (2010).

[5] Reilly, D. J. *et al.* Measurement of Temporal Correlations of the Overhauser Field in a Double Quantum Dot. *Physical Review Letters* **101**, 236803 (2008).

[6] Dial, O. E. *et al.* Supplement: Charge noise spectroscopy using coherent exchange oscillations in a singlet-triplet qubit. *Physical Review Letters* **110**, 1–4 (2013).

[7] Cerfontaine, P., Botzem, T., DiVincenzo, D. P. & Bluhm, H. High-Fidelity Single-Qubit Gates for Two-Electron Spin Qubits in GaAs. *Physical Review Letters* **113**, 150501 (2014).

[8] Kelly, J. *et al.* Optimal Quantum Control Using Randomized Benchmarking. *Physical Review Letters* **112**, 240504 (2014).

[9] Green, T., Uys, H. & Biercuk, M. J. High-Order Noise Filtering in Nontrivial Quantum Logic Gates. *Physical Review Letters* **109**, 020501 (2012).

[10] Petta, J. R. *et al.* Coherent manipulation of coupled electron spins in semiconductor quantum dots. *Science* **309**, 2180–2184 (2005).

[11] Reilly, D. J., Marcus, C. M., Hanson, M. P. & Gossard, A. C. Fast single-charge sensing with a rf quantum point contact. *Applied Physics Letters* **91**, 89–92 (2007).

[12] Takahashi, M., Bartlett, S. D. & Doherty, A. C. Tomography of a spin qubit in a double quantum dot. *Physical Review A* **88**, 022120 (2013).

[13] Barthel, C., Reilly, D., Marcus, C., Hanson, M. & Gossard, A. Rapid Single-Shot Measurement of a Singlet-Triplet Qubit. *Physical Review Letters* **103**, 160503 (2009).

[14] Dobrovitski, V. V., de Lange, G., Ristè, D. & Hanson, R. Bootstrap Tomography of the Pulses for Quantum Control. *Physical Review Letters* **105**, 077601 (2010).

[15] Barends, R. *et al.* Superconducting quantum circuits at the surface code threshold for fault tolerance. *Nature* **508**, 500–503 (2014).

[16] Magesan, E., Gambetta, J. M. & Emerson, J. Characterizing quantum gates via randomized benchmarking. *Physical Review A* **85**, 042311 (2012).

[17] Wallman, J. J., Barnhill, M. & Emerson, J. Robust characterization of leakage errors. *New Journal of Physics* **18**, 043021 (2016).

[18] Magesan, E. *et al.* Efficient Measurement of Quantum Gate Error by Interleaved Randomized Benchmarking. *Physical Review Letters* **109**, 080505 (2012).

[19] Epstein, J. M., Cross, A. W., Magesan, E. & Gambetta, J. M. Investigating the limits of randomized benchmarking protocols. *Physical Review A* **89**, 062321 (2014).
